# Supplementary material for: On Using Certified Training towards Empirical Robustness
Source: arXiv:2410.01617 source file (2025-03-24)
Supplement: Supplementary file 1 [file appendix-forwabs-co.tex]

While our Forwabs regularization relates to the L1 regularization focusing on the absolute value of the weights we show in \figref{fig:forwabs-cifar10-8} that 
they have different effects on CO. L1 regularization either fails to prevent CO for lower regularization coefficients, or 
lead to a constant classifier for higher coefficients while Forwabs prevents CO for higher coefficients and only fails for very low coefficients.
This failure mode can further be mitigated by scheduling the regularization, increase $\lambda$ during the training.

\begin{figure}
\begin{subfigure}{0.32\textwidth}
  \centering
  \includegraphics[width=.9\linewidth]{plots/fgsm-L1.pdf}
  \caption{L1 regularization}
  \label{plot-fgsm-L1}
\end{subfigure}
\begin{subfigure}{0.32\textwidth}
  \centering
  \includegraphics[width=.9\linewidth]{plots/forwabs.pdf}
  \caption{Forwabs regularization}
  \label{plot-fgsm-forwabs}
\end{subfigure}
\begin{subfigure}{0.32\textwidth}
  \centering
  \includegraphics[width=.9\linewidth]{plots/forwabs-sched.pdf}
  \caption{Forwabs scheduled regularization}
  \label{plot-fgsm-ibp}
\end{subfigure}
\caption{
    Comparison of L1 regularization, Forwabs regularization, Forwabs with coefficient scheduling regularization.
    L1. CO or leads to a constant classifier. 
    Forwabs prevents CO except for $\lambda \in \{1e-13,1e-15\}$.
    Forwabs with coefficient scheduling consistently prevents CO.
}
\label{fig:forwabs-cifar10-8}
\end{figure}

For further experiments we use the forwabs regularization on top of N-FGSM. 
We tune $\lambda$ on CIFAR10 $\epsilon = 24/255$, and on SVHN $\epsilon = 12/255$, the largest $\epsilon$ we use, the most challenging 
for CO. We find that N-FGSM in fact suffers from CO at this $\epsilon$ setting, while N-FGSM with Forwabs does not.
We believe it was not reported in previous work as the typical number of runs used (3) was not enough to observe the phenomenon.
We train on 5 seeds for each setting to improve the robustness of our results.
\begin{figure}
\begin{subfigure}{0.32\textwidth}
  \centering
  \includegraphics[width=.9\linewidth]{plots/forwabs_vs_nfgsm-cifar10-16_255.pdf}
  \caption{CIFAR10 $\epsilon = 16/255$}
  \label{plot-forwabs-nfgsm-cifar10-16}
\end{subfigure}
\begin{subfigure}{0.32\textwidth}
  \centering
  \includegraphics[width=.9\linewidth]{plots/forwabs_vs_nfgsm-cifar10-20_255.pdf}
  \caption{CIFAR10 $\epsilon = 20/255$}
  \label{plot-forwabs-nfgsm-cifar10-20}
\end{subfigure}
\begin{subfigure}{0.32\textwidth}
  \centering
  \includegraphics[width=.9\linewidth]{plots/forwabs_vs_nfgsm-cifar10-24_255.pdf}
  \caption{CIFAR10 $\epsilon = 24/255$}
  \label{plot-forwabs-nfgsm-cifar10-24}
\end{subfigure}
\caption{
    Comparison of N-FGSM and N-FGSM with Forwabs regularization on CIFAR10.
    N-FGSM suffers from CO at $\epsilon = 20/255$ while N-FGSM with Forwabs does not.
}
\end{figure}
